# Supplementary material for: CKAA: Cross-subspace Knowledge Alignment and Aggregation for Robust Continual Learning
Source: arXiv:2507.09471 source file (2026-08-20)
Supplement: Supplementary file 1 [file X_suppl.tex]

\clearpage
\setcounter{page}{1}
\maketitlesupplementary

\setcounter{equation}{0}
\setcounter{table}{0}

\appendix
% \section{}

\begin{table*}
\centering
\caption{Model performance under different adapter widths.}\label{tab: varying_width}
\vspace{-3.5mm}
\begin{adjustbox}{max width=1.0\textwidth}
\begin{tabular}{c|c|c|cc|cc}
\hline
\multirow{2}*{Width} & \multirow{2}*{Params} & \multirow{2}*{Flops} & \multicolumn{2}{c|}{10s-ImageNetA} & \multicolumn{2}{c}{10s-ImageNetR} \\
\cline{4-7}
& & & 
Last-acc $\uparrow$ &Avg-acc $\uparrow$ & Last-acc $\uparrow$ & Avg-acc $\uparrow$\\
\hline
2 & 0.42M (0.48\%) & 17.09GMac & 63.40\tsb{\(\pm\)0.66} & 71.84\tsb{\(\pm\)0.46} & 81.63\tsb{\(\pm\)0.70} & 86.93\tsb{\(\pm\)0.04} \\
4 & 0.83M (0.96\%) & 17.16GMac & 63.84\tsb{\(\pm\)0.47} & \textbf{72.15}\tsb{\(\pm\)0.76} & 82.04\tsb{\(\pm\)0.20} & 87.02\tsb{\(\pm\)0.07} \\
8 & 1.66M (1.93\%) & 17.31GMac &  \textbf{64.03}\tsb{\(\pm\)1.06} & 72.09\tsb{\(\pm\)0.14}  & 81.77\tsb{\(\pm\)0.75} & 86.96\tsb{\(\pm\)0.07} \\
16 & 3.32M (3.86\%) & 17.60GMac & 63.56\tsb{\(\pm\)0.32} & 71.27\tsb{\(\pm\)1.15} & 82.06\tsb{\(\pm\)1.09} & 87.03\tsb{\(\pm\)0.35} \\
32 & 6.64M (7.72\%) & 18.18GMac & 63.27\tsb{\(\pm\)0.74} & 71.33\tsb{\(\pm\)1.13} & 82.15\tsb{\(\pm\)0.47} & \textbf{87.21}\tsb{\(\pm\)0.13} \\
64 & 13.28M (15.44\%) & 19.34GMac & 63.53\tsb{\(\pm\)0.66} & 71.11\tsb{\(\pm\)1.03} & \textbf{82.41}\tsb{\(\pm\)0.13} & 87.20\tsb{\(\pm\)0.35} \\
\hline
\end{tabular}
\end{adjustbox}
\vspace{-2mm}
\end{table*}

\begin{table*}
\centering
\caption{Analysis of memory and computational overhead.}\label{tab: analysis_memory}
\vspace{-3.5mm}
\begin{adjustbox}{max width=1.0\textwidth}
\begin{tabular}{c|c|c|c|cc}
\hline
\multirow{2}*{Method} &
\multirow{2}*{Params} & \multirow{2}*{Training Flops} & 
\multirow{2}*{Inference Flops} &
\multicolumn{2}{c}{10s-ImageNetA} \\
\cline{5-6}
& & & & Last-acc $\uparrow$ & Avg-acc $\uparrow$\\
\hline
frozen ViT & 86M & 16.88GMac & 16.88GMac & 46.01\tsb{\(\pm\)0.92} & 56.51\tsb{\(\pm\)0.70} \\
+ $\mathcal{P}_{sh}$ & +0.04M (0.05\%) & 17.00GMac & 17.00GMac & 53.83\tsb{\(\pm\)0.37} & 63.93\tsb{\(\pm\)1.08} \\ 
CKAA-  & +0.46M (0.53\%) & 17.01GMac & (17.00+17.09)GMac & 63.40\tsb{\(\pm\)0.66} & \textbf{71.84}\tsb{\(\pm\)0.46}\\ 
CKAA & +13.32M (15.48\%) & 17.23GMac & (17.00+19.34)GMac & \textbf{63.53}\tsb{\(\pm\)0.66} & 71.11\tsb{\(\pm\)1.03} \\ 
\hline
\end{tabular}
\end{adjustbox}
\vspace{-2mm}
\end{table*}

\begin{table*}
\centering
\caption{Comparison with existing methods on performance and memory.}\label{tab: comparison_with_sota_memory}
\vspace{-3.5mm}
\begin{adjustbox}{max width=1.0\textwidth}
\begin{tabular}{c|c|c|cc|cc}
\hline
\multirow{2}*{Methods} & \multirow{2}*{Venue} & \multirow{2}*{Params} & \multicolumn{2}{c|}{10s-ImageNetA} & \multicolumn{2}{c}{10s-ImageNetR} \\
\cline{4-7}
& & & 
Last-acc $\uparrow$ &Avg-acc $\uparrow$ & Last-acc $\uparrow$ & Avg-acc $\uparrow$\\
\hline
DualPrompt \cite{dualpromptECCV22} & ECCV-22 & +0.25M (0.29\%) & 53.19\tsb{\(\pm\)0.74} &64.59\tsb{\(\pm\)0.08} & 69.10\tsb{\(\pm\)0.62} & 74.28\tsb{\(\pm\)0.66} \\
CODA \cite{codaCVPR23} & CVPR-23 & +3.84M (4.46\%)
& 52.08\tsb{\(\pm\)0.12} &  63.92\tsb{\(\pm\)0.12} & 
73.31\tsb{\(\pm\)0.50} & 78.47\tsb{\(\pm\)0.53} \\
SSIAT \cite{ssaitCVPR24} & CVPR-24 & +1.19M (1.38\%) & 
62.43\tsb{\(\pm\)1.63} & 70.83\tsb{\(\pm\)1.63}  & 
79.38\tsb{\(\pm\)0.59} & 83.63\tsb{\(\pm\)0.43} \\
\hline
CKAA- & -- & +0.46M (0.53\%) & 63.40\tsb{\(\pm\)0.66} & \textbf{71.84}\tsb{\(\pm\)0.46} & 81.63\tsb{\(\pm\)0.70} & 86.93\tsb{\(\pm\)0.04} \\
CKAA & -- & +13.32M (15.48\%) & \textbf{63.53}\tsb{\(\pm\)0.66} & 71.11\tsb{\(\pm\)1.03} & \textbf{82.41}\tsb{\(\pm\)0.13} & \textbf{87.20}\tsb{\(\pm\)0.35} \\
\hline
\end{tabular}
\end{adjustbox}
\vspace{-2mm}
\end{table*}

\begin{table*}[t]
\centering
\caption{Task-by-task accuracy of the \emph{\textbf{challenging samples}} on 10s-ImageNetA.}\label{tab: incorrect-acc-imageneta}
\vspace{-2mm}
\begin{adjustbox}{max width=1.0\textwidth}
\begin{tabular}{l|ccccccccc}
\hline
Methods & Ses.2 & Ses.3 & Ses.4 & Ses.5 & Ses.6 & Ses.7 & Ses.8 & Ses.9 & Ses.10 \\
\hline
\multicolumn{9}{l}{\textit{CKAA with frozen pre-trained task-shared network.}}\\
\hline
pre-trained backbone & 0.00\tsb{\(\pm\)0.00}	& 0.00\tsb{\(\pm\)0.00}& 0.00\tsb{\(\pm\)0.00}&	0.00\tsb{\(\pm\)0.00}&	0.00\tsb{\(\pm\)0.00}	&0.00\tsb{\(\pm\)0.00}	&0.00\tsb{\(\pm\)0.00}	&0.00\tsb{\(\pm\)0.00}	&0.00\tsb{\(\pm\)0.00}\\
+ TC-MoA 
&43.26\tsb{\(\pm\)5.96}	
&44.84\tsb{\(\pm\)5.08} 
&43.67\tsb{\(\pm\)1.45} 
&39.47\tsb{\(\pm\)2.20}	
&36.09\tsb{\(\pm\)2.26}	
&35.01\tsb{\(\pm\)2.87}
&32.29\tsb{\(\pm\)1.01}
&31.00\tsb{\(\pm\)1.75}	
&30.20\tsb{\(\pm\)1.46}\\
+ TC-MoA + CA 
&52.20\tsb{\(\pm\)2.80}	
&51.74\tsb{\(\pm\)4.33}	
&48.49\tsb{\(\pm\)1.28}	
&46.61\tsb{\(\pm\)1.56}	
&43.99\tsb{\(\pm\)1.64}	
&41.93\tsb{\(\pm\)2.53}	
&40.51\tsb{\(\pm\)0.51}	
&39.19\tsb{\(\pm\)0.41}	
&37.88\tsb{\(\pm\)0.47}\\
+ TC-MoA + FA 
&43.72\tsb{\(\pm\)7.96}	
&48.07\tsb{\(\pm\)7.06}	
&47.08\tsb{\(\pm\)2.65}	
&43.17\tsb{\(\pm\)2.16}	
&41.81\tsb{\(\pm\)2.52}	
&37.80\tsb{\(\pm\)3.44}	
&36.68\tsb{\(\pm\)3.04}	
&34.73\tsb{\(\pm\)1.53}	
&33.76\tsb{\(\pm\)1.24}\\
+ TC-MoA + DKA 
&\textbf{53.99}\tsb{\(\pm\)6.41}
&\textbf{53.06}\tsb{\(\pm\)2.95}	
&\textbf{52.60}\tsb{\(\pm\)1.86}	
&\textbf{49.65}\tsb{\(\pm\)0.27}	
&\textbf{47.33}\tsb{\(\pm\)2.52}	
&\textbf{45.11}\tsb{\(\pm\)2.82}	
&\textbf{44.54}\tsb{\(\pm\)0.87}	
&\textbf{42.87}\tsb{\(\pm\)0.89}	
&\textbf{42.01}\tsb{\(\pm\)0.66} \\
\hline
\multicolumn{9}{l}{\textit{CKAA with learnable visual prompt-based task-shared network.}}\\
\hline
$\mathcal{P}_{sh}$ & 0.00\tsb{\(\pm\)0.00}	& 0.00\tsb{\(\pm\)0.00}& 0.00\tsb{\(\pm\)0.00}&	0.00\tsb{\(\pm\)0.00}&	0.00\tsb{\(\pm\)0.00}	&0.00\tsb{\(\pm\)0.00}	&0.00\tsb{\(\pm\)0.00}	&0.00\tsb{\(\pm\)0.00}	&0.00\tsb{\(\pm\)0.00}\\
+ TC-MoA & 23.90\tsb{\(\pm\)5.54}	& 19.97\tsb{\(\pm\)1.67}& 17.62\tsb{\(\pm\)1.23}&	14.82\tsb{\(\pm\)2.42}&	13.29\tsb{\(\pm\)1.13}	&12.31\tsb{\(\pm\)0.33}	&12.48\tsb{\(\pm\)1.05}	&11.41\tsb{\(\pm\)0.5}	&10.48\tsb{\(\pm\)0.22} \\
+ TC-MoA + CA & 30.48\tsb{\(\pm\)5.96} &	29.59\tsb{\(\pm\)0.88} &	30.80\tsb{\(\pm\)6.53} &	28.56\tsb{\(\pm\)5.17} &	27.54\tsb{\(\pm\)2.62} &	27.36\tsb{\(\pm\)3.25} & 25.97\tsb{\(\pm\)1.60} &	25.50\tsb{\(\pm\)1.08} &	25.68\tsb{\(\pm\)0.39} \\
+ TC-MoA + FA & 20.96\tsb{\(\pm\)4.42} &	21.41\tsb{\(\pm\)4.48} & 21.95\tsb{\(\pm\)3.96} &	19.60\tsb{\(\pm\)2.12} &	17.94\tsb{\(\pm\)1.73} &	17.59\tsb{\(\pm\)3.21} &	17.25\tsb{\(\pm\)2.05} & 16.81\tsb{\(\pm\)1.57} & 16.43\tsb{\(\pm\)1.52}\\
+ TC-MoA + DKA & \textbf{35.76}\tsb{\(\pm\)0.93} & \textbf{33.75}\tsb{\(\pm\)8.83} & \textbf{36.02}\tsb{\(\pm\)2.03} & \textbf{31.84}\tsb{\(\pm\)2.85} & \textbf{31.28}\tsb{\(\pm\)2.78} & \textbf{29.91}\tsb{\(\pm\)2.85} & \textbf{29.25}\tsb{\(\pm\)1.42} & \textbf{28.31}\tsb{\(\pm\)1.97} & \textbf{27.71}\tsb{\(\pm\)0.53} \\
\hline
\end{tabular}
\end{adjustbox}
\vspace{-2mm}
\end{table*}

\begin{table*}[t]
\centering
\caption{Task-by-task accuracy of the \emph{\textbf{easy samples}} on 10s-ImageNetA.}\label{tab: correct-acc-imageneta}
\vspace{-2mm}
\begin{adjustbox}{max width=1.0\textwidth}
\begin{tabular}{l|ccccccccc}
\hline
Methods & Ses.2 & Ses.3 & Ses.4 & Ses.5 & Ses.6 & Ses.7 & Ses.8 & Ses.9 & Ses.10 \\
\hline
\multicolumn{9}{l}{\textit{CKAA with frozen pre-trained task-shared network.}}\\
\hline
pre-trained backbone 
&67.05\tsb{\(\pm\)3.05}
&67.15\tsb{\(\pm\)0.96}
&69.63\tsb{\(\pm\)1.68}	
&71.60\tsb{\(\pm\)2.15}	
&72.61\tsb{\(\pm\)3.42}	
&73.43\tsb{\(\pm\)2.46}	
&74.12\tsb{\(\pm\)1.52}	
&72.56\tsb{\(\pm\)1.93}	
&72.57\tsb{\(\pm\)1.84} \\
+ TC-MoA 
&79.50\tsb{\(\pm\)3.98}
&82.11\tsb{\(\pm\)3.68}
&82.65\tsb{\(\pm\)1.49}
&83.54\tsb{\(\pm\)1.81}
&82.73\tsb{\(\pm\)0.99}
&82.48\tsb{\(\pm\)0.69}
&82.91\tsb{\(\pm\)2.30}
&82.53\tsb{\(\pm\)1.06}	
&82.41\tsb{\(\pm\)1.36} \\
+ TC-MoA + CA 
&81.92\tsb{\(\pm\)2.65}
&85.46\tsb{\(\pm\)1.61}
&86.08\tsb{\(\pm\)1.03}	
&87.17\tsb{\(\pm\)1.66}	
&87.25\tsb{\(\pm\)1.13}	
&86.24\tsb{\(\pm\)0.63}	
&86.09\tsb{\(\pm\)1.34}	
&85.92\tsb{\(\pm\)1.70}	
&86.36\tsb{\(\pm\)1.68} \\
+ TC-MoA + FA 
&81.07\tsb{\(\pm\)3.75}
&82.75\tsb{\(\pm\)3.30}	
&82.68\tsb{\(\pm\)1.20}
&84.89\tsb{\(\pm\)0.40}
&83.85\tsb{\(\pm\)1.63}	
&84.49\tsb{\(\pm\)1.52}	
&84.97\tsb{\(\pm\)0.86}	
&84.76\tsb{\(\pm\)2.38}	
&84.35\tsb{\(\pm\)2.39} \\
+ TC-MoA + DKA 
&\textbf{83.12}\tsb{\(\pm\)1.31}
&\textbf{86.40}\tsb{\(\pm\)1.86}	
&\textbf{86.19}\tsb{\(\pm\)0.99}	
&\textbf{88.81}\tsb{\(\pm\)1.34}	
&\textbf{87.79}\tsb{\(\pm\)1.34}	
&\textbf{86.78}\tsb{\(\pm\)0.75}	
&\textbf{86.89}\tsb{\(\pm\)2.12}	
&\textbf{86.87}\tsb{\(\pm\)2.89}	
&\textbf{86.83}\tsb{\(\pm\)3.30} \\
\hline
\multicolumn{9}{l}{\textit{CKAA with learnable visual prompt-based task-shared network.}}\\
\hline
$\mathcal{P}_{sh}$ 
&81.92\tsb{\(\pm\)2.49}	
&83.42\tsb{\(\pm\)2.79}	
&85.05\tsb{\(\pm\)3.00}	
&85.80\tsb{\(\pm\)2.99}	
&85.86\tsb{\(\pm\)2.48}	
&85.14\tsb{\(\pm\)1.72}	
&85.79\tsb{\(\pm\)1.49}	
&85.45\tsb{\(\pm\)1.79}	
&85.98\tsb{\(\pm\)1.17} \\
+ TC-MoA 
&79.01\tsb{\(\pm\)3.99}
&80.84\tsb{\(\pm\)2.24}	
&83.49\tsb{\(\pm\)4.47}	
&84.31\tsb{\(\pm\)1.51} 
&84.60\tsb{\(\pm\)1.27}	
&83.62\tsb{\(\pm\)0.48}
&83.07\tsb{\(\pm\)0.64}	
&82.33\tsb{\(\pm\)1.43}	
&82.85\tsb{\(\pm\)1.97} \\
+ TC-MoA + CA 
&80.10\tsb{\(\pm\)9.33}
&84.19\tsb{\(\pm\)3.20}	
&86.26\tsb{\(\pm\)3.78}	
&85.54\tsb{\(\pm\)1.66}	
&86.09\tsb{\(\pm\)1.42}	
&86.64\tsb{\(\pm\)3.07}	
&86.84\tsb{\(\pm\)0.39}	
&85.71\tsb{\(\pm\)0.49}
&85.76\tsb{\(\pm\)0.50}\\
+ TC-MoA + FA 
&80.22\tsb{\(\pm\)1.81}
&82.35\tsb{\(\pm\)2.26}	
&84.26\tsb{\(\pm\)0.55}	
&85.22\tsb{\(\pm\)1.74}	
&85.30\tsb{\(\pm\)1.09}
&85.02\tsb{\(\pm\)2.25}	
&83.91\tsb{\(\pm\)1.05}	
&84.34\tsb{\(\pm\)1.93}	
&83.49\tsb{\(\pm\)2.56} \\
+ TC-MoA + DKA 
&\textbf{82.81}\tsb{\(\pm\)4.11} 	
&\textbf{85.13}\tsb{\(\pm\)1.71} 	
&\textbf{86.95}\tsb{\(\pm\)2.04} 	
&\textbf{87.76}\tsb{\(\pm\)2.66} 	
&\textbf{88.07}\tsb{\(\pm\)1.11} 	
&\textbf{87.39}\tsb{\(\pm\)1.38} 	
&\textbf{87.23}\tsb{\(\pm\)0.85} 	
&\textbf{86.08}\tsb{\(\pm\)0.81} 	
&\textbf{86.51}\tsb{\(\pm\)0.52} \\
\hline
\end{tabular}
\end{adjustbox}
\vspace{-3mm}
\end{table*}

\begin{table}[t]
\centering
\caption{Experimental results on 10s-CUB-200. }\label{tab: cub200}
\vspace{-2mm}
\begin{adjustbox}{max width=0.48\textwidth}
\begin{tabular}{l|l|cc}
\hline
\multirow{1}*{Method} & \multirow{1}*{Venue}
& Last-acc $\uparrow$ &Avg-acc $\uparrow$\\
\hline
L2P \cite{l2pCVPR22} & CVPR-22 & 67.02\tsb{\(\pm\) 1.90} &79.62\tsb{\(\pm\) 1.60}\\
DualPrompt \cite{dualpromptECCV22} & ECCV-22 & 68.48\tsb{\(\pm\) 0.47} &80.59\tsb{\(\pm\) 1.50}\\
CODAPrompt \cite{codaCVPR23} & CVPR-23 & 77.23\tsb{\(\pm\) 1.12} &81.90\tsb{\(\pm\) 0.85} \\
LAE \cite{laeICCV23} & ICCV-23 & 80.97\tsb{\(\pm\) 0.51}	& 87.22\tsb{\(\pm\) 1.21} \\
SLCA \cite{slcaICCV23} & ICCV-23 & 84.68\tsb{\(\pm\) 0.09}&	90.77\tsb{\(\pm\) 0.79} \\
Adam-adapter \cite{adamIJCV2024} & IJCV-24 & 85.84\tsb{\(\pm\) 0.08} &	91.33\tsb{\(\pm\)0.49} \\
% EvoPrompt \cite{evopromptAAAI24} & \\
% InfLoRA \cite{infloraCVPR24} &\\
% CPrompt \cite{cpromptCVPR24} &\\
EASE \cite{easeCVPR24} & CVPR-24 & \multicolumn{1}{l}{86.81} & \multicolumn{1}{l}{92.23} \\
SSIAT \cite{ssaitCVPR24} & CVPR-24 & \underline{88.75}\tsb{\(\pm\) 0.38} &\underline{93.00}\tsb{\(\pm\) 0.90} \\
VPT-NSP$^{\dag}$ \cite{vptnspNIPS-24} & NIPS-24 & 83.08\tsb{\(\pm\) 0.75} & 90.32\tsb{\(\pm\) 0.62}\\
STAR-prompt \cite{star-promptECCV24} & ECCV-24 & 84.10\tsb{\(\pm\) 0.28} & --\\
CoFiMA \cite{CoFiMAECCV24} & ECCV-24 & 87.11\tsb{\(\pm\)0.56} & 91.87\tsb{\(\pm\)0.69}\\
\hline
\textbf{CKAA (Ours)} & -- & \textbf{89.48}\tsb{\(\pm\)0.46} &  \textbf{93.34}\tsb{\(\pm\)0.26} \\ 
\hline
\end{tabular}
\end{adjustbox}
\vspace{-2mm}
\end{table}

\begin{table}[t]
\centering
\caption{Experimental results on 10s-StanfordCars. }\label{tab: stanfordcars}
\vspace{-2mm}
\begin{adjustbox}{max width=0.48\textwidth}
\begin{tabular}{l|l|cc}
\hline
\multirow{1}*{Method} & \multirow{1}*{Venue}
& Last-acc $\uparrow$ &Avg-acc $\uparrow$\\
\hline
L2P \cite{l2pCVPR22} & CVPR-22 & 60.39\tsb{\(\pm\)1.99} & 71.92\tsb{\(\pm\)1.12}\\
DualPrompt \cite{dualpromptECCV22} & ECCV-22 & 57.27\tsb{\(\pm\)0.34} & 70.36\tsb{\(\pm\)2.33}\\
ESN \cite{esnAAAI23} & AAAI-23 & 56.91\tsb{\(\pm\)0.56} & 72.82\tsb{\(\pm\)0.79} \\
CODAPrompt \cite{codaCVPR23} & CVPR-23 & 62.24\tsb{\(\pm\)0.14} & 73.28\tsb{\(\pm\)0.93} \\
CPrompt \cite{cpromptCVPR24} & CVPR-24 & \underline{66.77}\tsb{\(\pm\)0.37} & \underline{76.81}\tsb{\(\pm\)0.27} \\
\hline
\textbf{CKAA (Ours)} & -- & \textbf{80.92}\tsb{\(\pm\)0.08} &  \textbf{87.32}\tsb{\(\pm\)0.90} \\ 
\hline
\end{tabular}
\end{adjustbox}
% \vspace{-2mm}
\end{table}

\begin{table*}[t]
\centering
\caption{Ablation Studies of the learnable visual prompt-based task-shared network on ImageNetR and ImageNetA. }\label{tab: ablation-study-shared}
\vspace{-2mm}
\begin{adjustbox}{max width=1.0\textwidth}
\begin{tabular}{c|cccc|cc|cc|cc}
\hline
\multirow{2}*{Idx} & 
\multirow{2}*{$\mathcal{P}_{sh}$} &
% \multirow{2}*{$\mathcal{A}^t_{sp}$} &
\multirow{2}*{TC-MoA} & 
\multirow{2}*{CA} & 
\multirow{2}*{FA} &
\multicolumn{2}{c|}{10s-ImageNetR} &
\multicolumn{2}{c|}{10s-ImageNetA} & 
\multicolumn{2}{c}{20s-ImageNetR}\\
\cline{6-11}
& {} & {} & {} & {}
& Last-acc $\uparrow$ &Avg-acc $\uparrow$
& Last-acc $\uparrow$ &Avg-acc $\uparrow$
& Last-acc $\uparrow$ &Avg-acc $\uparrow$\\
\hline
\multicolumn{11}{l}{\textit{CKAA with frozen pre-trained task-shared network.}}\\
\hline
1& -- & -- & -- & -- & 65.65\tsb{\(\pm\)0.58} & 72.82\tsb{\(\pm\)0.67} & 46.01\tsb{\(\pm\)0.92} & 56.51\tsb{\(\pm\)0.70} & 63.67\tsb{\(\pm\)0.68} & 71.56\tsb{\(\pm\)1.14}\\
2& -- & \checkmark & -- & -- & 76.72\tsb{\(\pm\)0.61} & 83.14\tsb{\(\pm\)0.32} & 53.92\tsb{\(\pm\)0.85} & 64.16\tsb{\(\pm\)0.18} & 73.91\tsb{\(\pm\)0.35} & 81.15\tsb{\(\pm\)0.32}\\
3& -- & \checkmark & \checkmark & -- & 79.77\tsb{\(\pm\)0.12} & 85.09\tsb{\(\pm\)0.24} & 59.71\tsb{\(\pm\)0.20} & 68.55\tsb{\(\pm\)0.32}  & 78.65\tsb{\(\pm\)0.27} & 84.52\tsb{\(\pm\)0.41}\\
4& -- & \checkmark & -- & \checkmark & 78.54\tsb{\(\pm\)0.39} & 84.36\tsb{\(\pm\)0.28} &  57.12\tsb{\(\pm\)1.75} & 65.68\tsb{\(\pm\)0.25} & 75.58\tsb{\(\pm\)0.19} & 82.43\tsb{\(\pm\)0.76} \\
5& -- & \checkmark & -- & \checkmark & \textbf{81.56}\tsb{\(\pm\)0.13} & \textbf{86.63}\tsb{\(\pm\)0.13} & \textbf{62.49}\tsb{\(\pm\)1.53} & \textbf{70.59}\tsb{\(\pm\)0.56} & \textbf{79.86}\tsb{\(\pm\)0.32} & \textbf{85.33}\tsb{\(\pm\)0.52}\\
\hline
\multicolumn{11}{l}{\textit{CKAA with learnable visual prompt-based task-shared network.}}\\
\hline
6& \checkmark & -- & -- & -- & 77.95\tsb{\(\pm\)0.22} & 83.44\tsb{\(\pm\)0.40} & 53.83\tsb{\(\pm\)0.37} & 63.93\tsb{\(\pm\)1.08} & 75.69\tsb{\(\pm\)0.62} & 81.87\tsb{\(\pm\)0.56}\\
7& \checkmark & \checkmark & -- & -- & 79.14\tsb{\(\pm\)0.21} & 85.04\tsb{\(\pm\)0.33} & 54.33\tsb{\(\pm\)0.87} & 64.43\tsb{\(\pm\)1.22} & 76.88\tsb{\(\pm\)0.57} & 82.91\tsb{\(\pm\)0.52}\\
8& \checkmark & \checkmark & \checkmark & -- & 81.80\tsb{\(\pm\)0.38} & 86.59\tsb{\(\pm\)0.18} & 61.29\tsb{\(\pm\)0.46} & 69.31\tsb{\(\pm\)1.16} & 80.18\tsb{\(\pm\)0.42} & 85.75\tsb{\(\pm\)0.24}\\
9& \checkmark & \checkmark & -- & \checkmark & 79.74\tsb{\(\pm\)0.34} & 85.29\tsb{\(\pm\)0.19} & 58.13\tsb{\(\pm\)0.20} & 66.59\tsb{\(\pm\)0.84} & 77.82\tsb{\(\pm\)0.55} & 83.71\tsb{\(\pm\)0.39}\\
10& \checkmark & \checkmark & \checkmark & \checkmark & 
\textbf{82.41}\tsb{\(\pm\)0.13} & \textbf{87.20}\tsb{\(\pm\)0.35} & \textbf{63.53}\tsb{\(\pm\)0.66} &  \textbf{71.11}\tsb{\(\pm\)1.03} &
\textbf{80.98}\tsb{\(\pm\)0.35} & \textbf{86.28}\tsb{\(\pm\)0.18}\\
\hline
\end{tabular}
\end{adjustbox}
% \vspace{-3mm}
\end{table*}

\section{The Whole Training and Inference Process}

\begin{algorithm}[!t] 
\caption{Training process for $t_c$-th task}  
\label{alg::training}
\begin{algorithmic}[1]
\REQUIRE The $t_c$-th training dataset $\mathcal{D}_{t_c}$, the pre-trained backbone $\mathcal{F}$, the task-shared prompts $\mathcal{P}_{sh}$, the task-specific adapter $\mathcal{A}^{t_c}_{sp}$ for $t_c$-th task.
\ENSURE The optimized prompt $\mathcal{P}_{sh}$ and adapter $\mathcal{A}^{t_c}_{sp}$,
the unified classifier $g^{t_c}$.
\STATE \textbf{Initialization}:
Randomly initialize adapters in $\mathcal{A}^{t_c}_{sp}$; Randomly initialize classifier $g^{t_c}$.
\IF{$t_c=1$}
\STATE Randomly initialize prompts in $\mathcal{P}^{sh}$.
\ENDIF
\FOR{$\{\mathbf{x}_i, y(\mathbf{x}_i)\}_{i=1}^{B}$ \textbf{in} $\mathcal{D}_{t_c}$}
\STATE Extract shared features $\mathcal{C}_{sh} = \{\mathbf{f}_i\}_{i=1}^B$ through the task-shared network, where $\mathbf{f}_i = \mathcal{F}(\mathbf{x}_i; \mathcal{P}_{sh})$;
\STATE Extract specific features $\mathcal{C}_{sp} = \{\mathbf{z}_i\}_{i=1}^B$ through the specific adapters, where $\mathbf{f}_i = \mathcal{F}(\mathbf{x}_i; \mathcal{P}_{sh}, \mathcal{A}^{t_c}_{sp})$;
\STATE Compute $\mathcal{L}_{ce}$ through Eq.\textcolor{iccvblue}{3};\\
\IF{$t_c > 1$}
\STATE \textcolor[rgb]{0.1, 0.6, 0.8}{// The Feature-level Alignment}
\STATE Extract features $\{\mathbf{\tilde{z}}_i^{t_c \rightarrow t_p}\}_{i=1}^{B}$ of images from current batch within the previous feature subspaces:\\
$\mathbf{\tilde{z}}_i^{t_c \rightarrow t_p} = \mathcal{F}(\mathbf{x}_i^{t_c}; \mathcal{P}_{sh}, \mathcal{A}^{t_p}_{sp})$;\\
\STATE Compute the Cross-Subspace Feature Alignment loss $\mathcal{L}_{csfa}$ as Eq.\textcolor{iccvblue}{4};\\
\STATE \textcolor[rgb]{0.1, 0.6, 0.8}{// The Classifier-level Alignment}
\STATE Sample previous features $\mathcal{S}_{sh} = \{\tilde{\mathbf{f}}_i\}_{i=1}^{B_s}$ from Gaussian distributions $\cup_{t \leq t_c-1} \mathcal{G}_{k,t}$;\\
\STATE Modeling affinities $\mathbf{G}$ between current and previous data as Eq.\textcolor{iccvblue}{5};\\
\STATE Construct simulated features $\mathcal{S}_{sp} = \{\tilde{\mathbf{f}}_i\}_{i=1}^{B_s}$ based on affinities $\mathbf{G}$ as Eq.\textcolor{iccvblue}{6};\\
\STATE Build the unified feature set $\mathcal{U}$ and compute the classifier-level alignment loss $\mathcal{L}_{cu}$ as Eq.\textcolor{iccvblue}{7};\\
\ENDIF
\STATE Compute total loss $\mathcal{L}$ as Eq.\textcolor{iccvblue}{9};
\ENDFOR
\STATE \textcolor[rgb]{0.1, 0.6, 0.8}{//Optimization}
\STATE Update visual prompts $\mathcal{P}_{sh}$ in the null space of the previous feature space;\\
\STATE Update task-specific adapters $\mathcal{A}^{t_c}_{sp}$;\\
\IF{$t_c > 1$}
\STATE Update classifier $g^{t_c}$;
\ENDIF
\STATE \textcolor[rgb]{0.1, 0.6, 0.8}{//Gaussian Modeling}
\FOR{class $y$ \textbf{in} $\mathcal{Y}^{t_c}$}
\STATE Extract the centroid and covariance of all image features belonging to class $y$;\\
\STATE Build an Gaussian Distribution $\mathcal{G}_{y,t_c}$ for class $y$;\\
\ENDFOR
\STATE Aggregate the classifier weights to build $g^u$ as Eq.\textcolor{iccvblue}{8}.
\end{algorithmic}
\end{algorithm}

\begin{algorithm}
\caption{Inference process after $t_c$-th task}  
\label{alg::inference}
\begin{algorithmic}[1]
    % \textbf{Input:\\}
\REQUIRE The inference dataset $\{\mathbf{x}_i\}_{i=1}^{N}$, the pre-trained backbone $\mathcal{F}$, the optimized prompts $\mathcal{P}_{sh}$ and adapters $\{\mathcal{A}^t_{sp}\}_{t=1}^{t_c}$, the aggregated unified classifier $g^u$.
\ENSURE The prediction $\{\hat{k}_i\}_{i=1}^N$ for $\{\mathbf{x}_i\}_{i=1}^{N}$.
\FOR{$\mathbf{x}_i$ \textbf{in} $\{\mathbf{x}_i\}_{i=1}^N$}
\STATE Extract shared feature $\mathbf{f}_i$ from the task-shared network, where $\mathbf{f}_i = \mathcal{F}(\mathbf{x}_i; \mathcal{P}_{sh})$;
\STATE Derive task-confidence scores $\{P_t(t|\mathbf{f}_i)\}_{t=1}^{t_c}$ of feature $\mathbf{f}_i$ as Eq.\textcolor{iccvblue}{10} and Eq.\textcolor{iccvblue}{11};
\STATE Obtain the aggregated feature $\hat{\mathbf{z}}_i$ from TC-MoA based on the task-confidence scores $\{P_t(t|\mathbf{f}_i)\}_{t=1}^{t_c}$, where $\hat{\mathbf{z}}_i=\mathcal{F}(\mathbf{x}_i; \mathcal{P}_{sh}, \{\mathcal{A}^t_{sp}\}_{t=1}^{t_c}, \{\alpha^t_i\}_{t=1}^{t_c})$;
\STATE Obtain the final prediction $\hat{k}_i$ following Eq.\textcolor{iccvblue}{13}.
\ENDFOR
\end{algorithmic}
\end{algorithm}

\noindent The whole training process of our CKAA is outlined in Alg.\ref{alg::training}.
When $t_c$-th task arrives, our training framework includes learning a set of task-shared prompts $\mathcal{P}_{sh}$, a set of task-specific adapters $\mathcal{A}^{t_c}_{sp}$ and a task-adaptive classifier $g^{t_c}$.
Our training scheme includes the standard cross-entropy, the classifier-level, and feature-level knowledge alignment.
The whole inference process is shown in Alg.\ref{alg::inference}.
The inference of our CKAA includes deriving the task-confidence scores through the task-shared network and aggregating task-specific knowledge through the proposed TC-MoA.

\section{Experimental Results}\label{supp: experiments}

\subsection{Analysis of the additional memory and computational overhead}

We conduct experiments to analyze the impact of adapter widths on 10s-ImageNetA and 10s-ImageNetR datasets, the results are shown in Tab.\ref{tab: varying_width}.
Decreasing the adapter width results in slight performance degradation on 10s-ImageNetR, while it exhibits negligible impact on the performance of 10s-ImageNetA.
Notably, our method performs well even with a width of 2, referred to as `CKAA-'.
We also analyze the additional memory and computational overhead brought by our task-shared and specific components, as shown in Tab.\ref{tab: analysis_memory}.
While the specific modules indeed bring significant performance improvements, their inference requires two forward processes, inevitably increasing FLOPs due to the task-specific design—a challenge common to all task-specific frameworks, 
$e.g.$, L2P \cite{l2pCVPR22}, CODA \cite{codaCVPR23} and EASE \cite{easeCVPR24}.

To demonstrate both the effectiveness and efficiency of our framework, we compare our CKAA- and CKAA with existing methods on both performance and memory in Tab.\ref{tab: comparison_with_sota_memory}.
\textbf{\emph{Our efficient version, `CKAA-', achieves superior performances with a parameter count comparable to SOTAs.}}

\subsection{Analysis of the Impact of Misleading Task-ids}

We conduct ablation studies on 10s-ImageNetA to analyze the effectiveness of our proposed CKAA in enhancing the model's robustness against misleading task-ids.
Specifically, we divide the testing samples into two subsets:
(1) \emph{\textbf{Challenging samples}}: These are misclassified by the task recognizer into incorrect classes under incorrect tasks;
(2) \emph{\textbf{Easy samples}}: These are classified into the classes under correct task-ids.
The task recognizer struggles to estimate reliable task-ids for these \textbf{\emph{challenging samples}} while allocating inappropriate sub-modules.
We report the task-by-task accuracy of these two types of samples, respectively.
The results are shown in Tab.\ref{tab: incorrect-acc-imageneta} and Tab.\ref{tab: correct-acc-imageneta}.
The upper part of Tab.\ref{tab: incorrect-acc-imageneta} and Tab.\ref{tab: correct-acc-imageneta} utilizes the pre-trained backbone as the task-recognizer, whereas the lower part introduces our learnable visual prompt-based task-shared network to serve as the task recognizer.

As shown in Tab.\ref{tab: incorrect-acc-imageneta}, the proposed TC-MoA and DKA effectively improve the prediction accuracy for these samples, delivering more reliable predictions for features under inappropriate task-specific sub-modules.
Since our learnable task-shared network (the lower part) encapsulates sufficient downstream task information, the samples it fails to distinguish are inherently more challenging for the model.
Therefore, the accuracy in the lower part of Tab.\ref{tab: incorrect-acc-imageneta} is lower compared to the upper part.
However, our proposed method still achieves significant improvement in the classification accuracy of these challenging samples.
Meanwhile, the results of our method in Tab.\ref{tab: correct-acc-imageneta} do not show a decline for samples deemed easy by the task recognizer, demonstrating that our CKAA improves the accuracy of challenging samples without compromising performance on easy samples.
To sum up, the core improvement of our CKAA lies in maintaining the prediction accuracy for easy samples while enhancing the model's accuracy in identifying challenging samples under incorrect task-ids.
Additionally, these results confirm that images can still generate meaningful features even when processed by incorrect sub-modules, further highlighting the critical importance of enhancing the model's robustness under misleading task-ids in PEFT-based CIL methods.

\subsection{Comparison with Existing Methods on Fine-Grained CIL Learning}

We evaluate our method on the fine-grained datasets CUB-200 \cite{CUB}
and StanfordCars \cite{stanfordcars2013} to demonstrate its effectiveness in fine-grained CIL classification.
CUB-200 \cite{CUB} contains 11,788 images of 200 bird species with fine-grained class labels.
StanfordCars \cite{stanfordcars2013} is a fine-grained car dataset including 196 classes and 16185 car images. 
Following existing methods \cite{ssaitCVPR24, adamIJCV2024, cpromptCVPR24}, we evaluate our method under the 10-split setting.
The experiment results on CUB-200 and StanfordCars are exhibited in Tab.\ref{tab: cub200} and Tab.\ref{tab: stanfordcars}, respectively.
Our method exhibits superior performance, outperforming the state-of-the-art SSIAT by 0.73\% Last-acc on CUB-200 and 14.15\% Last-acc on StanfordCars.
The results demonstrate the robustness of our method against the catastrophic forgetting of fine-grained knowledge.

\subsection{Parameter Analysis}

We conduct experiments to analyze the impact of the hyper-parameters in our method on 10s-ImageNetR and 10s-ImageNetA benchmarks, including $\tau_f$ in Eq.\textcolor{iccvblue}{4}, $K_g$ and $\tau_g$ in Eq.\textcolor{iccvblue}{5}, $K_c$ in Eq.\textcolor{iccvblue}{10} and $\tau$ in Eq.\textcolor{iccvblue}{11}.

We first analyze the hyper-parameters in TC-MoA, including $K_c$ and $\tau$. 
The results are shown in Fig.\ref{fig: parameter-K_c} and Fig.\ref{fig: parameter-tau}.
$K_c$ is designed to select the Top-$K_c$ classes with the highest logits to compute the task-confidence scores.
Too small $K_c$ resulting in insufficient instance-class relationships and too large $K_c$ 
will introduce redundant classes with dissimilar semantics.
We set $K_c=10$ for ImageNetR and $K_c=20$ for ImageNetA based on experimental results in Fig.\ref{fig: parameter-K_c}.
$\tau$ is a temperature factor designed to control the smoothness of the task-confidence scores.
If $\tau=0$, it is equal to directly selecting one task-specific sub-module with the highest confidence for inference.
If $\tau \rightarrow +\infty$, it is equal to aggregate the task-specific knowledge through the average pooling operation.
We set $\tau=2.0$ for all datasets based on experimental results in Fig.\ref{fig: parameter-tau}.

Then we analyze the hyper-parameters in DKA, including $\tau_f$, $K_g$, and $\tau_g$.
The results are shown in Fig.\ref{fig: parameter-tau_f}, Fig.\ref{fig: parameter-K_g}, and Fig.\ref{fig: parameter-tau_g}.
$\tau_f$ is a temperature factor of the Cross Subspace Feature Alignment (CSFA) loss in Eq.\textcolor{iccvblue}{4}.
The change in hyper-parameter $\tau_f$ has a relatively notable impact on the model performance since it affects the convergence of our Cross-Subspace Feature Alignment (CSFA) loss.
Based on the results in Fig.\ref{fig: parameter-tau_f}, we set $\tau_f=0.05$ for both datasets. 
$K_g$ and $\tau_g$ are two parameters for modeling the affinities between current and previous data.
$K_g$ selects the nearest neighbors in the feature space and eliminates excessive redundant relationships.
$\tau_g$ is a temperature factor for computing similarities, the term $\exp(\mathbf{a}{\mathbf{b}}^{\top} / \tau_g)$ enlarges the similarity differences between different instances while ensuring they are positive values.
% Since the affinities are mainly determined by similarities between features in the shared space, the variations in these two hyperparameters have few impacts on the performance.
Based on Fig.\ref{fig: parameter-K_g} and Fig.\ref{fig: parameter-tau_g}, we set $K_g=20$ and $\tau_g=0.2$ for all datasets.

\begin{figure}[h]
\centering
\includegraphics[width=0.48\textwidth]{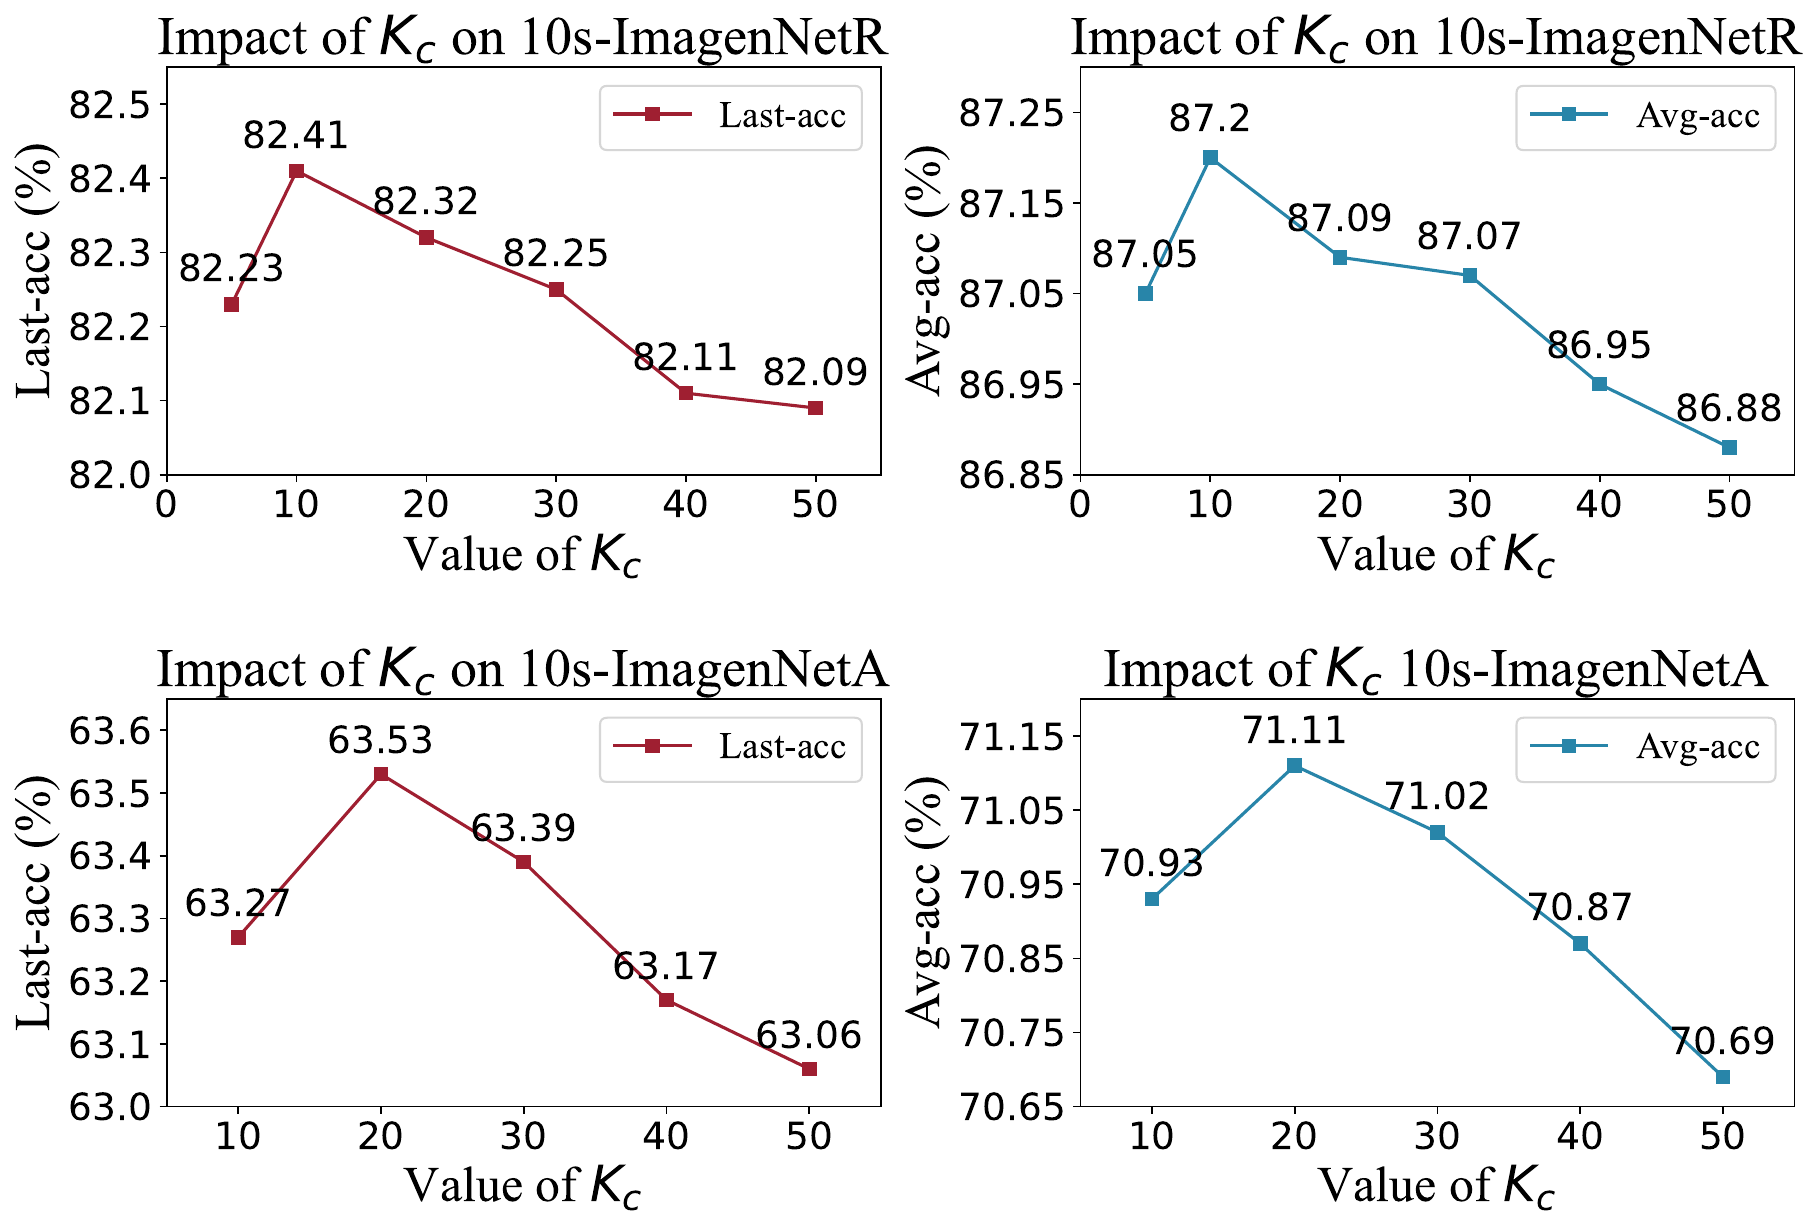}
\vspace{-7mm}
\caption{Parameter analysis of $K_c$ in Eq.\textcolor{iccvblue}{10}
}\label{fig: parameter-K_c}
\vspace{-2mm}
\end{figure}

\begin{figure}[h]
\centering
\includegraphics[width=0.48\textwidth]{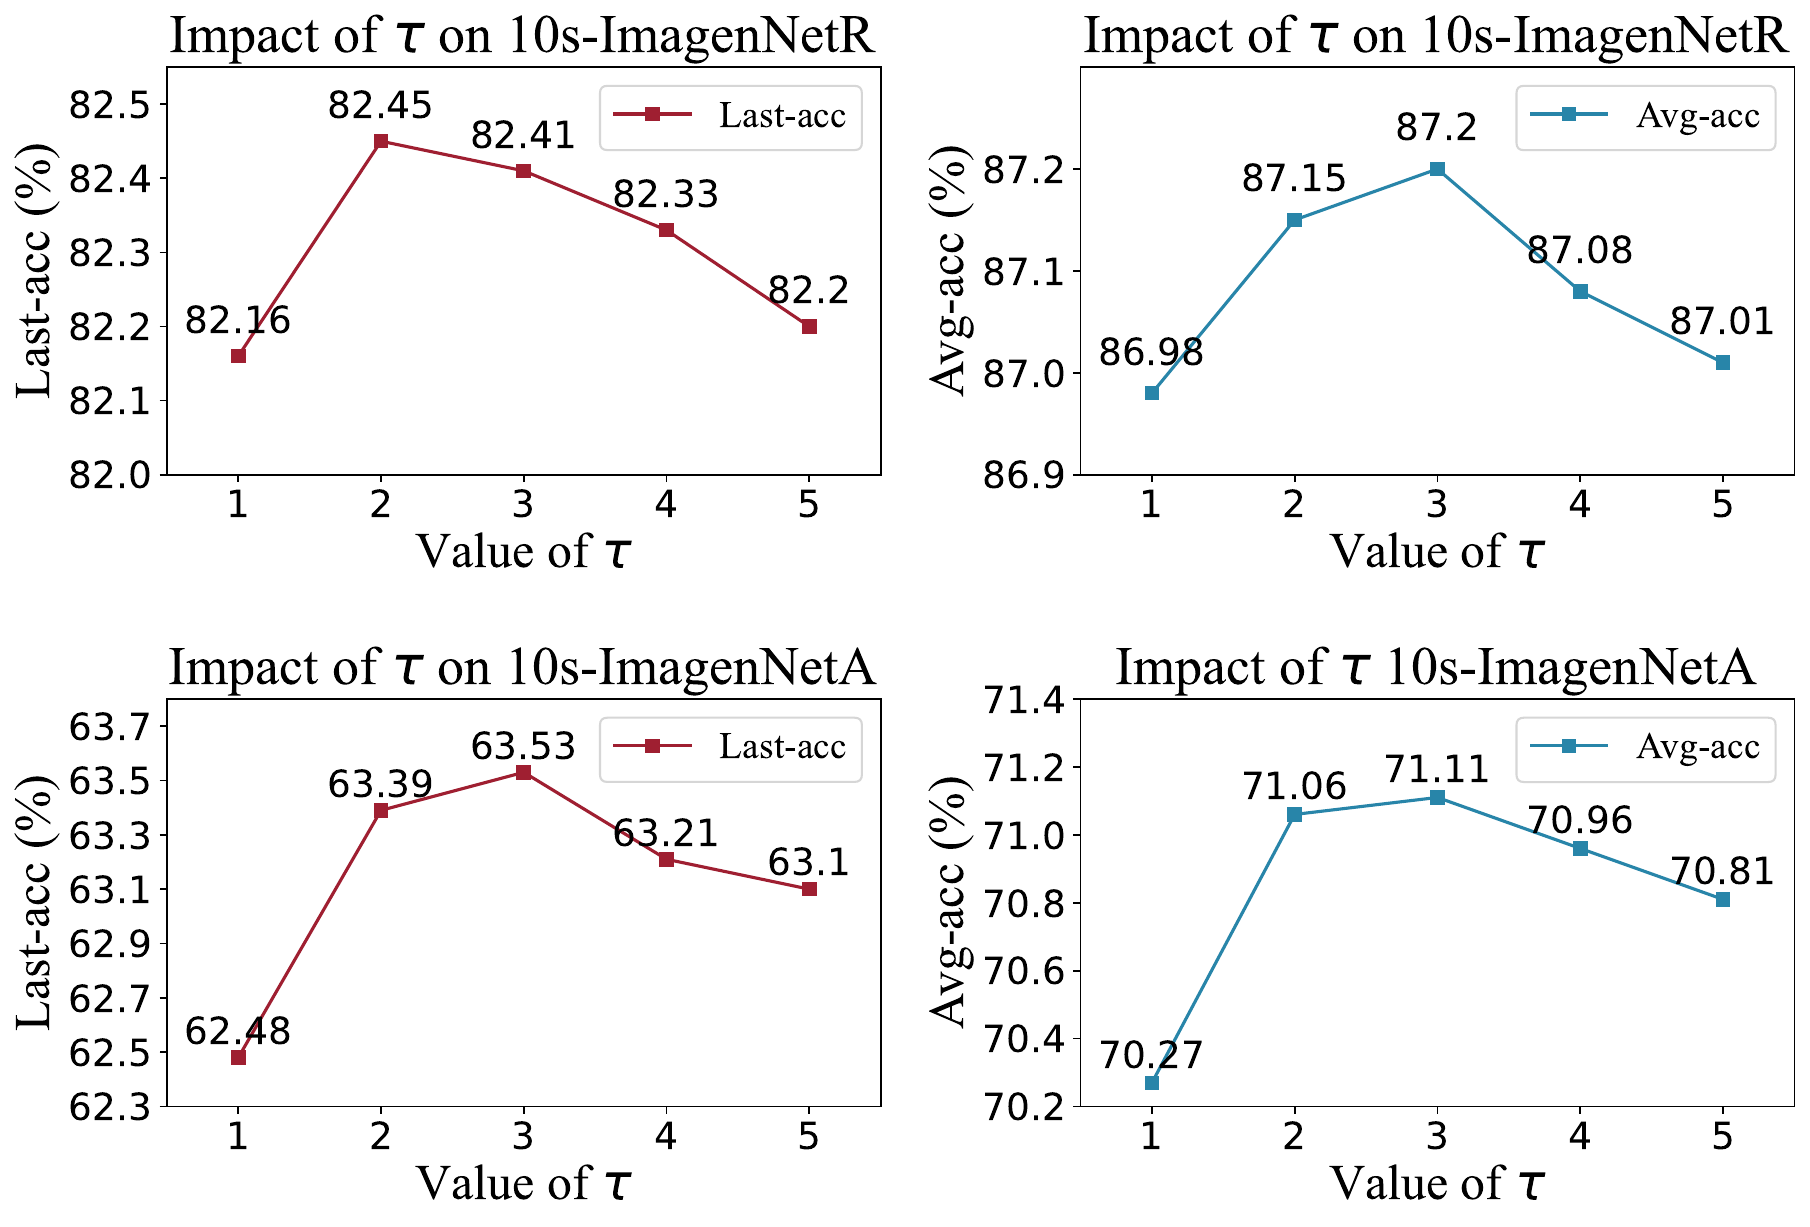}
\vspace{-7mm}
\caption{Parameter analysis of $\tau$ in Eq.\textcolor{iccvblue}{11}
}\label{fig: parameter-tau}
\vspace{-2mm}
\end{figure}

\begin{figure}[h]
\centering
\includegraphics[width=0.48\textwidth]{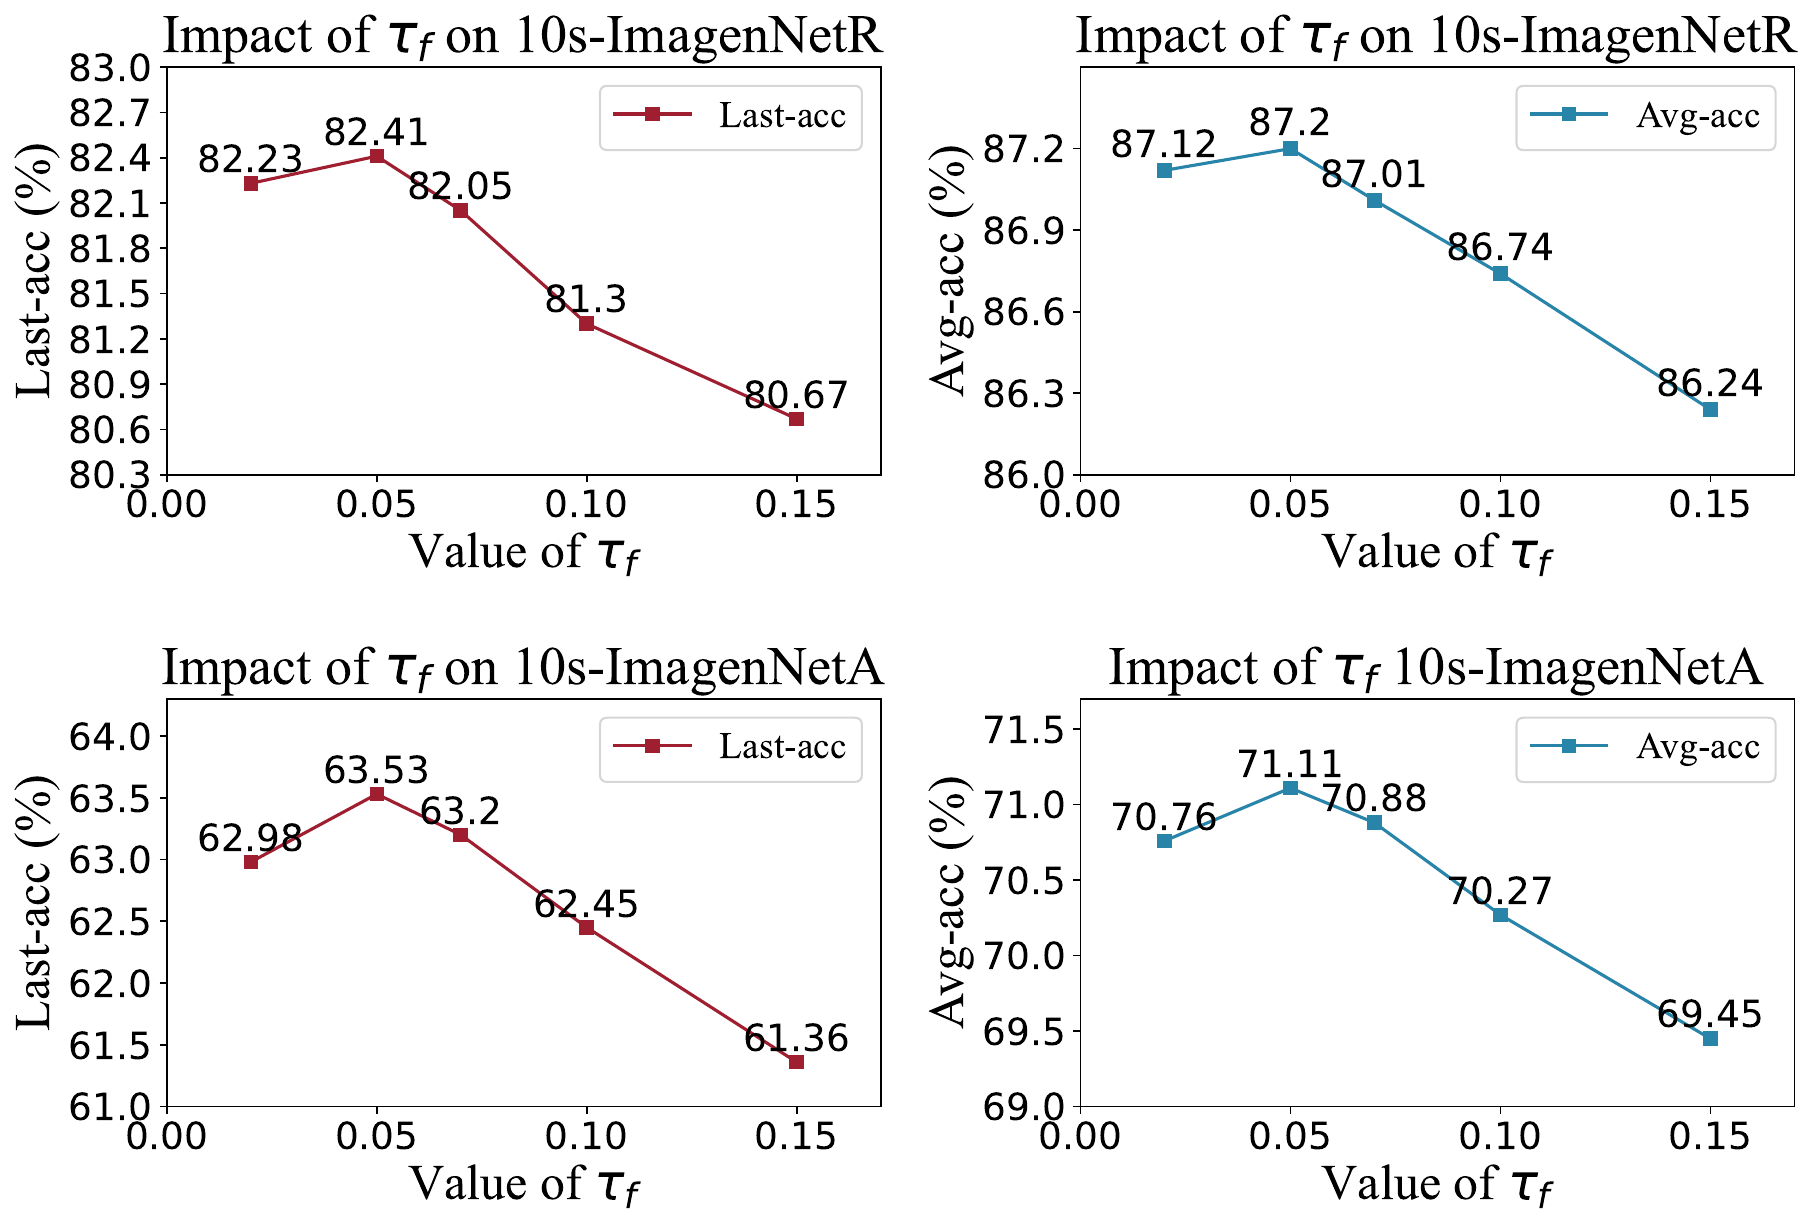}
\vspace{-7mm}
\caption{Parameter analysis of $\tau_f$ in Eq.\textcolor{iccvblue}{4}
}\label{fig: parameter-tau_f}
\vspace{-2mm}
\end{figure}

\begin{figure}[h]
\centering
\includegraphics[width=0.48\textwidth]{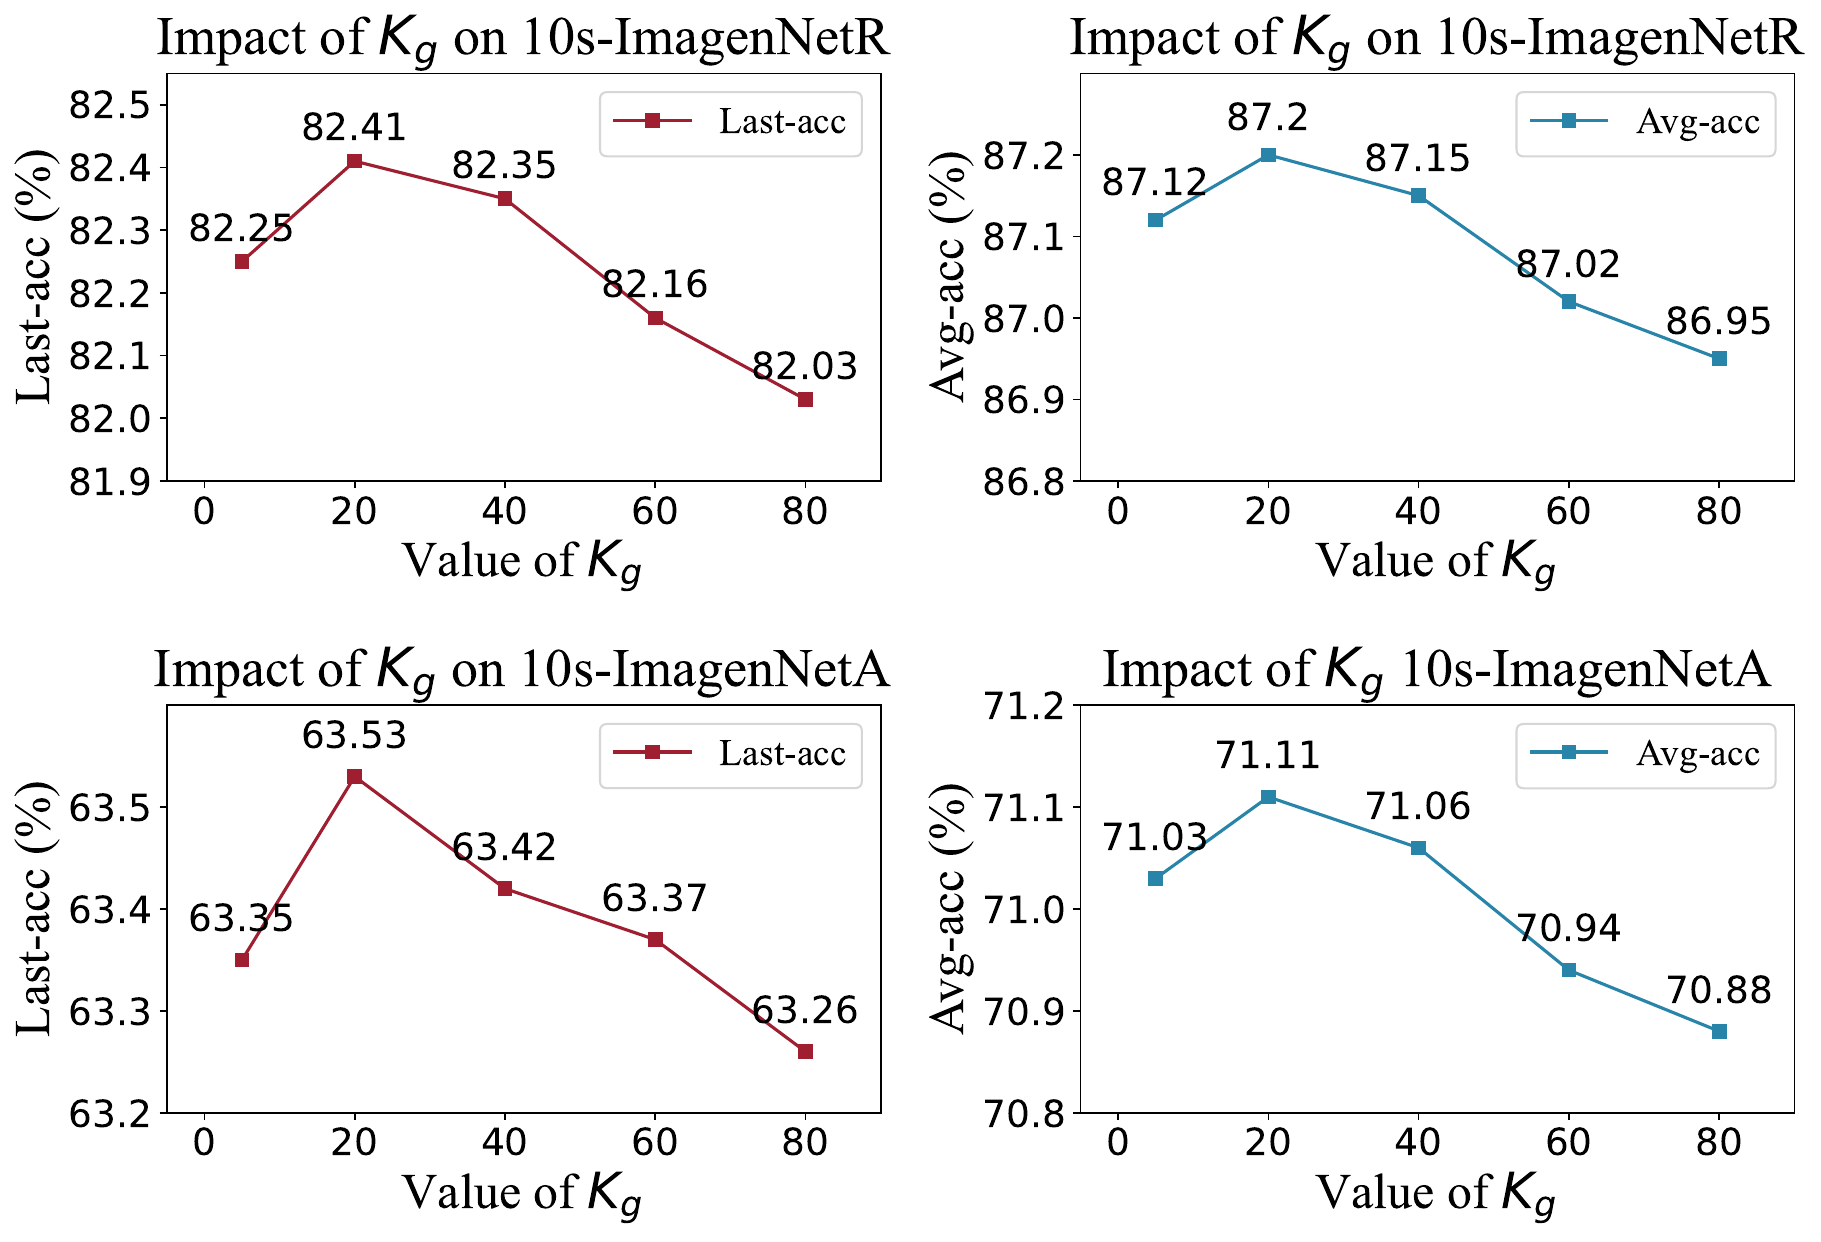}
\vspace{-7mm}
\caption{Parameter analysis of $K_g$ in Eq.\textcolor{iccvblue}{5}
}\label{fig: parameter-K_g}
\vspace{-2mm}
\end{figure}

\begin{figure}[h]
\centering
\includegraphics[width=0.48\textwidth]{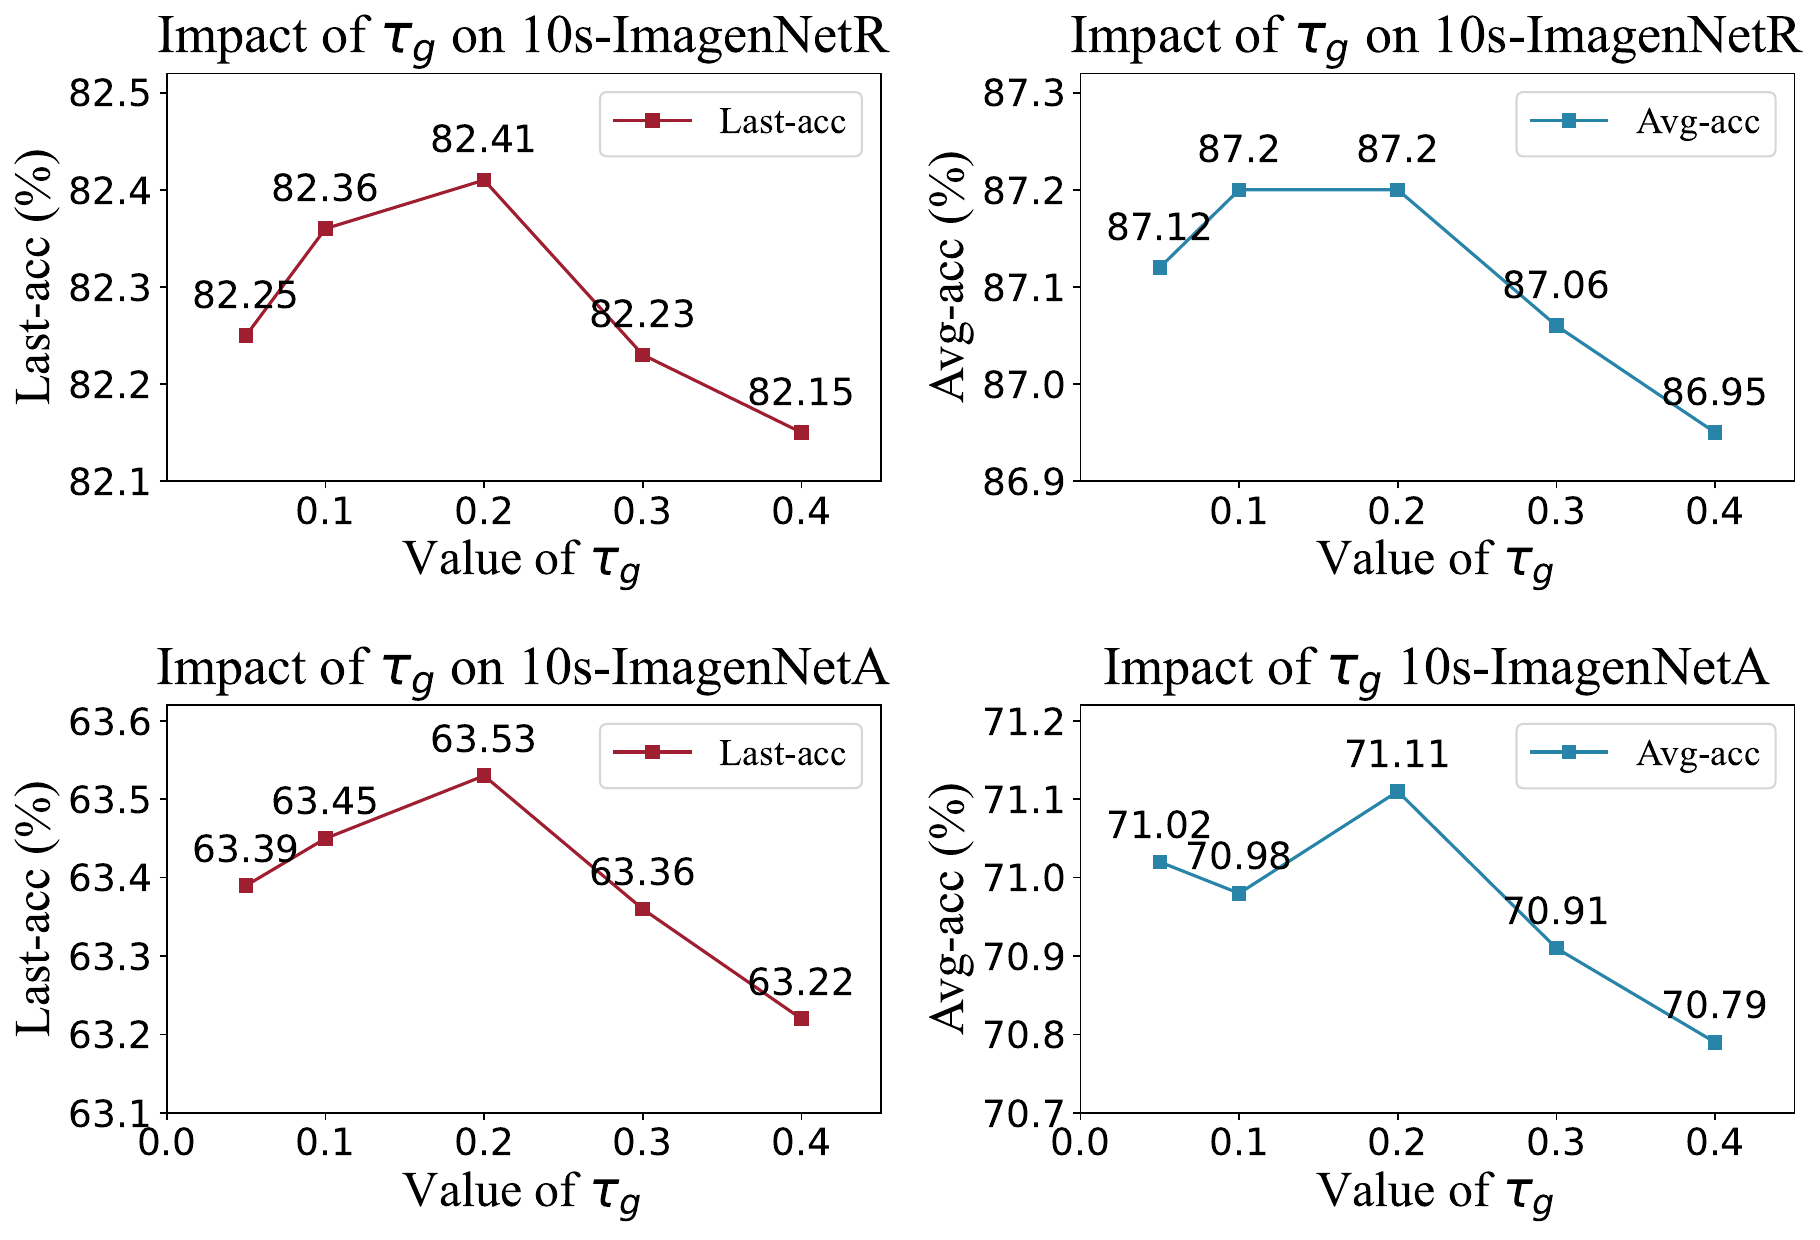}
\vspace{-7mm}
\caption{Parameter analysis of $\tau_g$ in Eq.\textcolor{iccvblue}{5}
}\label{fig: parameter-tau_g}
\vspace{-2mm}
\end{figure}

\subsection{Analysis of the Effectiveness of the Learnable Task-shared Network}

We conduct experiments on the learnable visual prompt-based task-shared network to demonstrate its effectiveness, the results are shown in Tab.\ref{tab: ablation-study-shared}.
Specifically, we directly replace the learnable task-shared network with the frozen pre-trained backbone.
As indicated in Tab.\ref{tab: ablation-study-shared},
the learnable visual prompts $\mathcal{P}_{sh}$ improves the model's Last-acc by 0.85\% and Avg-acc by 0.57\% on 10s-ImagenetR.
This improvement is mainly due to the learnable task-shared network’s ability to capture common knowledge across downstream datasets, compared to a frozen pre-trained backbone.
It results in more precise task identification during inference and more appropriate routing weights for aggregating task-specific knowledge in TC-MoA.
Meanwhile, the results in the upper section of Tab.\ref{tab: ablation-study-shared} further validate the effectiveness of our proposed DKA training scheme and TC-MoA inference approach.
With the frozen pre-trained backbone and a trainable classifier, the model achieves a limited performance of 65.65\% Last-acc and 72.82\% Avg-acc on 10s-ImagenetR.
Our TC-MoA obtains a significant performance gain of 11.07\% Last-acc and 10.32\% Avg-acc by incorporating task-specific knowledge of individual downstream tasks into the pre-trained backbone.
Our DKA further achieves an improvement of 4.84\% Last-acc and 3.49\% Avg-acc through the alignment across different task-specific subspaces.
The results demonstrate our DKA in enhancing the model's robustness against misleading task-ids.

\subsection{Experiments with Different ViT Models}

To demonstrate the generalizability of our CKAA, we conduct experiments on different ViTs with varying numbers of parameters, as shown in Tab.\ref{tab: varying_models}.
``CLIP, w/o text'' denotes the ViT-B/16 pre-trained by CLIP \cite{2021clip}, where the text encoder is discarded when fine-tuning on class-incremental learning datasets.
The results demonstrate the superiority of our CKAA.

\begin{table*}[h]
\centering
\vspace{-2mm}
\caption{Experiments with various ViT models.}\label{tab: varying_models}
\vspace{-3.5mm}
\begin{adjustbox}{max width=1.0\textwidth}
\begin{tabular}{c|c|c|cc|cc}
\hline
\multirow{2}*{Models} &
\multirow{2}*{Params} & 
\multirow{2}*{Methods} & 
\multicolumn{2}{c|}{10s-ImageNetA} &
\multicolumn{2}{c}{10s-ImageNetR} \\
\cline{4-7}
& & & Last-acc $\uparrow$ & Avg-acc $\uparrow$ & Last-acc $\uparrow$ & Avg-acc $\uparrow$\\
\hline
\multirow{2}*{ViT-Tiny} 
& \multirow{2}*{5.5M} 
& VPT-NSP \cite{vptnspNIPS-24} 
& 21.02\tsb{\(\pm\)1.27} 
& 31.20\tsb{\(\pm\)1.66}
& 47.82\tsb{\(\pm\)0.68} 
& 56.76\tsb{\(\pm\)0.77}\\
& & CKAA 
& \textbf{27.48}\tsb{\(\pm\)0.42} 
& \textbf{39.54}\tsb{\(\pm\)0.54}
& \textbf{58.49}\tsb{\(\pm\)0.14} 
& \textbf{67.65}\tsb{\(\pm\)1.08}\\
\hline
\multirow{2}*{ViT-Small} 
& \multirow{2}*{22M} 
& VPT-NSP \cite{vptnspNIPS-24} 
& 37.85\tsb{\(\pm\)0.60} 
& 48.37\tsb{\(\pm\)0.99} 
& 63.61\tsb{\(\pm\)0.34} 
& 71.08\tsb{\(\pm\)0.20}\\
& & CKAA 
& \textbf{47.07}\tsb{\(\pm\)0.40} 
& \textbf{57.60}\tsb{\(\pm\)1.21} 
& \textbf{73.77}\tsb{\(\pm\)0.15} 
& \textbf{81.05}\tsb{\(\pm\)1.09}\\
\hline
% ViT-Base & 86M & 
% \textbf{63.27}\tsb{\(\pm\)0.74} & 
% \textbf{71.33}\tsb{\(\pm\)1.13} & 
% 82.15\tsb{\(\pm\)0.47} & 
% 87.21\tsb{\(\pm\)0.13}\\
\multirow{2}*{ViT-Base (CLIP, w/o text)} 
& \multirow{2}*{86M} 
& VPT-NSP \cite{vptnspNIPS-24} 
& 51.07\tsb{\(\pm\)0.69} 
& 63.08\tsb{\(\pm\)0.88} 
& 80.55\tsb{\(\pm\)0.62} 
& 86.78\tsb{\(\pm\)0.32}\\
& & CKAA 
& \textbf{59.25}\tsb{\(\pm\)0.33} 
& \textbf{69.63}\tsb{\(\pm\)1.36} 
& \textbf{83.94}\tsb{\(\pm\)0.46} 
& \textbf{89.42}\tsb{\(\pm\)0.40}\\
\hline
\end{tabular}
\end{adjustbox}
\vspace{-2mm}
\end{table*}

\begin{figure}[!t]
\centering
\includegraphics[width=0.48\textwidth]{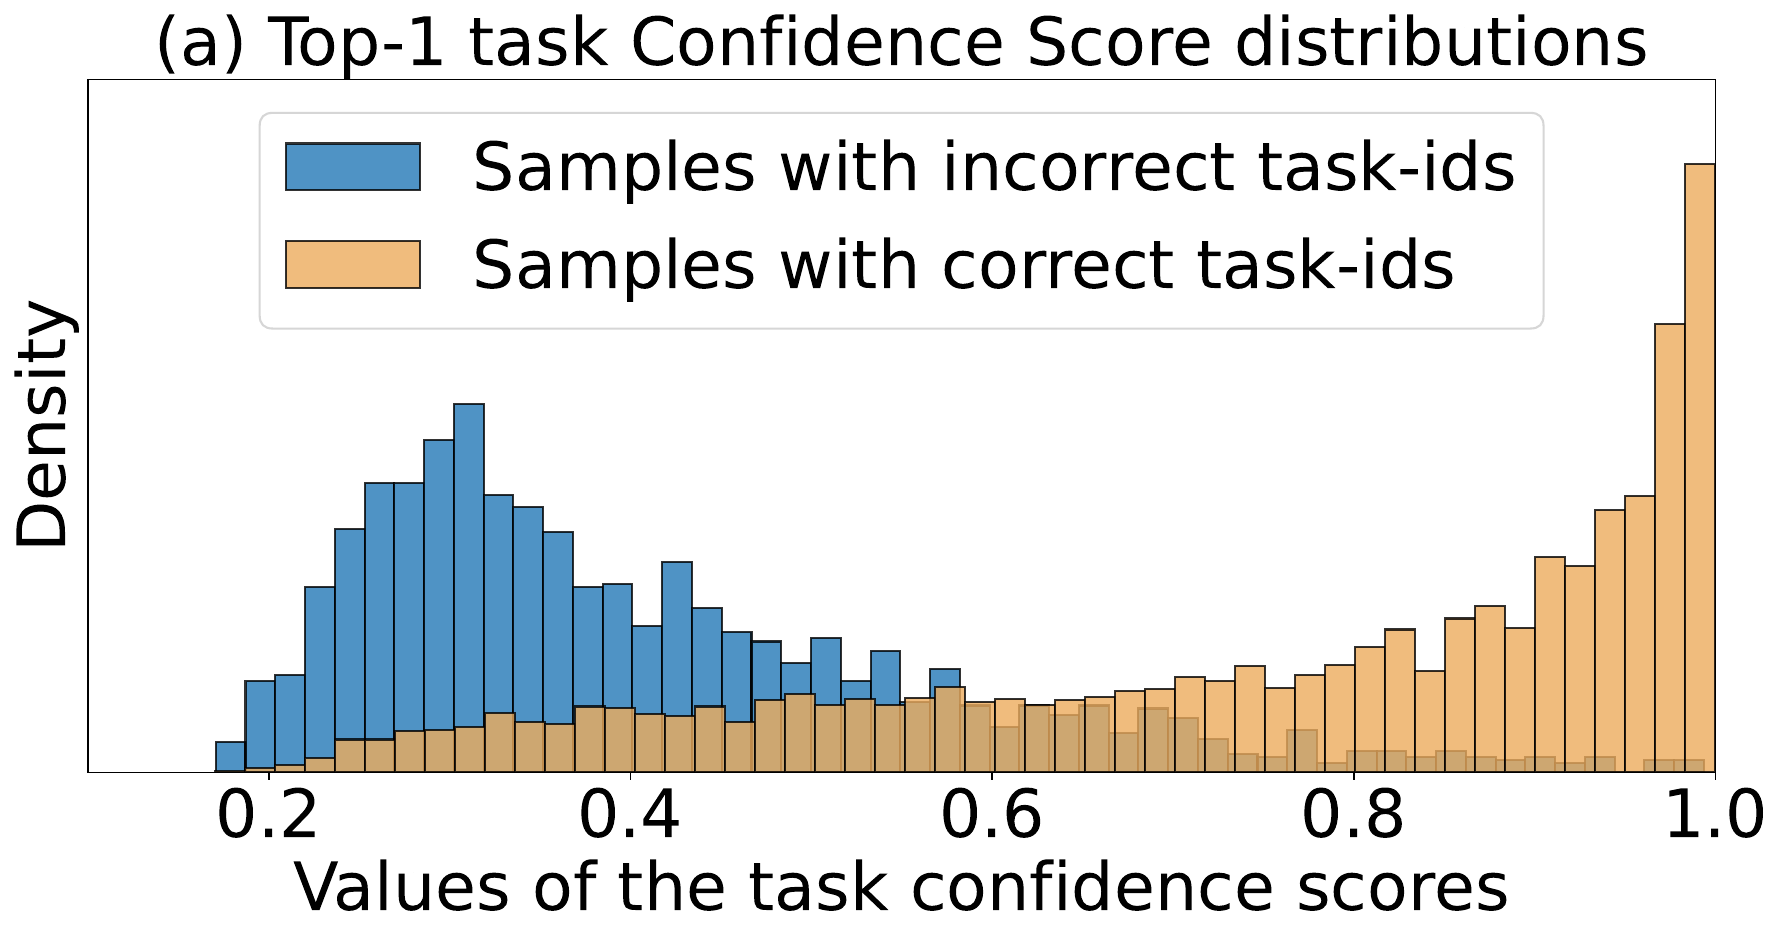}
\vspace{-5mm}
\caption{Visualization of the distributions of the top-1 task-confidence scores.
}\label{fig:visualization_tcmoa}
\vspace{-5mm}
\end{figure}

\subsubsection{Working Mechanism of the TC-MoA}

We visualize the top-1 confidence score distribution of samples with correct and incorrect task-ids in Fig.\ref{fig:visualization_tcmoa}.
For a test sample $\mathbf{x}_i^{t_g}$ from task $t_g$, its top-1 confidence score is denoted as $\alpha^{\hat{t}}_i$, where $\hat{t} = \arg\mathop{\max} \limits_{i} \alpha_i^t$.
For $\mathbf{x}_i^{t_g}$, if the predicted top-1 task matches its ground-truth task id, where $\hat{t} == t_g$, the sample is considered to have a correct prediction of task id.
As shown in Fig.\ref{fig:visualization_tcmoa}, samples with correct task-ids generally have higher top-1 scores.
Therefore, for samples predicted with correct task-ids, TC-MoA assigns a single task-specific module with high confidence while neglecting others, effectively acting as a \emph{\textbf{deterministic module selector}}.
For samples predicted with incorrect task-ids, TC-MoA adopts \emph{\textbf{a soft-label-like approach}}, softly compensating for the incorrect modules through intermediate features from potential correct modules.
Such a mechanism mitigates overconfidence in incorrect task-ids while preserving performance for correct ones, highlighting TC-MoA as a novel approach in handling incorrect task-ids during inference.

\subsection{Comparison with Traditional Methods}

Tab.\ref{tab: compare-with-traditional} presents a comparison between our CKAA method and traditional CIL methods on the ImageNet-R and ImageNet-A datasets under the 10-split setting. 
The results show the Last-acc and Avg-acc over three random seeds. 
On 10s-ImageNetR, CKAA achieves outstanding performance, with results of 82.41\% and 87.20\% in Last-acc and Avg-acc, respectively, substantially surpassing the best-competing method, Foster \cite{wang2022foster}, which reached Last-acc=75.87\% and Avg-acc=81.54\%. For 10s-ImageNetA, CKAA also demonstrates strong performance on this challenging dataset, achieving Last-acc=63.53\% and Avg-acc=71.11\%, which is significantly higher than Der \cite{expansion3}.
Overall, the results demonstrate the superior performance of our PEFT-based CKAA, which significantly outperforms learning from scratch.

\begin{table}[t]
\centering
\caption{Comparison to traditional CIL methods on ImageNetR and ImageNetA dataset under the 10-split setting. We report the averaged results over 3 random number seeds. The highest results are in bold and the second highest results are underlined.}\label{tab: compare-with-traditional}
\vspace{-2mm}
\begin{adjustbox}{max width=0.48\textwidth}
\begin{tabular}{l|cc|cc}
\hline
\multirow{2}*{Method} &
\multicolumn{2}{c|}{10s-ImageNetR} &
\multicolumn{2}{c}{10s-ImageNetA}\\
\cline{2-5}
& Last-acc $\uparrow$ &Avg-acc $\uparrow$
& Last-acc $\uparrow$ &Avg-acc $\uparrow$ \\
\hline
iCaRL \cite{iCaRL}   & 61.70\tsb{\(\pm\)0.56}  & 71.34\tsb{\(\pm\)0.67}  & 29.32\tsb{\(\pm\)2.36} & 40.11\tsb{\(\pm\)1.36}
\\
Foster \cite{wang2022foster}& 75.87\tsb{\(\pm\)0.38}  & 81.54\tsb{\(\pm\)0.82}  & 12.44\tsb{\(\pm\)17.45}   & 17.01\tsb{\(\pm\)20.44} \\
Der \cite{expansion3}   & 75.63\tsb{\(\pm\)0.86} & 81.13\tsb{\(\pm\)0.11} & 38.43\tsb{\(\pm\)2.39}  &  46.43\tsb{\(\pm\)3.29}       \\
Memo \cite{zhou2022model} & 65.38\tsb{\(\pm\)0.90} & 73.80\tsb{\(\pm\)0.86} & 28.45\tsb{\(\pm\)2.37}  & 40.27\tsb{\(\pm\)1.22}               \\
\hline
\textbf{CKAA (Ours)} & \textbf{82.41}\tsb{\(\pm\)0.13} & \textbf{87.20}\tsb{\(\pm\)0.35} & \textbf{63.53}\tsb{\(\pm\)0.66} & \textbf{71.11}\tsb{\(\pm\)1.03} \\ 
\hline
\end{tabular}
\end{adjustbox}
\vspace{-3mm}
\end{table}

% \subsection{Analysis of the Intermediate dimension in Adapters}

% We conduct experiments to study the impact of varying intermediate dimensions $\hat{d}$ in the task-specific adapters on 10s-ImageNetR, the results are shown in Tab.\ref{tab: dimension_imagenetr}.
% Based on the experimental results, we set the intermediate dimension to 64.
% Furthermore, the results demonstrate that our method is highly robust to the changes in intermediate dimensions.

% \begin{table}[t]
% \centering
% \caption{The impact of intermediate dimensions with different values on 10s-ImageNetR.}\label{tab: dimension_imagenetr}
% \vspace{-2mm}
% \begin{adjustbox}{max width=0.48\textwidth}
% \begin{tabular}{c|cc}
% \hline
% Dimension & Last-acc $\uparrow$ &Avg-acc $\uparrow$\\
% \hline
% 8 & 81.77\tsb{\(\pm\)0.75} & 86.93\tsb{\(\pm\)0.07} \\
% 16 & 82.06\tsb{\(\pm\)1.09} & 87.03\tsb{\(\pm\)0.35} \\
% 32 & 82.15\tsb{\(\pm\)0.47} & \textbf{87.21}\tsb{\(\pm\)0.13} \\
% 64 & \textbf{82.41}\tsb{\(\pm\)0.13} & 87.20\tsb{\(\pm\)0.35} \\
% \hline
% \end{tabular}
% \end{adjustbox}
% \vspace{-3mm}
% \end{table}

\section{More Details}\label{sec: supp_vptns}

% \vspace{-5mm}

\subsection{Details of Training Task-shared Prompts}

The task-shared prompts $\mathcal{P}_{sh}$ aims to explore the common knowledge across all downstream tasks through a fixed size of parameters while minimizing catastrophic forgetting.
Existing methods \cite{pgpICLR24, vptnspNIPS-24, GPM, OWM} build an orthogonal projector to project the gradients of learnable parameters into the direction orthogonal to the old feature spaces, which have demonstrated effectiveness in mitigating catastrophic forgetting.
Following these methods, we update the prompts in the null space of the previous feature space.
The output feature for $\mathbf{X}^t$ in task $\mathcal{D}_t$ is expected to
remain unchanged in the next task $\mathcal{D}_{t+1}$: 

\vspace{-2mm}
\begin{equation}\label{eq: null_space_definition}
    \mathcal{F}(\mathbf{X}^t; \mathcal{P}_{sh}^t) = 
    \mathcal{F}(\mathbf{X}^t; \mathcal{P}_{sh}^{t+1}),
\end{equation}

\noindent where $\mathcal{F}$ denotes the feature extractor. $\mathcal{P}_{sh}^t$ and $\mathcal{P}_{sh}^{t+1}$ is the prompt after training $t$-th and $t+1$-th task, respectively.
To achieve Eq.\ref{eq: null_space_definition}, we update the prompts in the null space of $\mathbf{Q}_{\mathbf{X}^t} {\mathbf{W}_k}^{\top}$ and 
$\mathbf{S}_{\mathbf{P}}$ following \cite{vptnspNIPS-24}.
Define the input $\mathbf{X}^t$ as consisting of $N$ tokens, each with $d$ dimensions, and the prompt $\mathbf{P}$ as consisting of $N_p$ tokens, each with $d$ dimensions.
$[\mathbf{Q}_{{\mathbf{X}^t}}, \mathbf{Q}_{\mathbf{P}}] = LN([\mathbf{X}^t, \mathbf{P}]) \mathbf{W}_q + \mathbf{b}_q \in \mathbb{R}^{(N+N_p) \times d}$ denotes the output of the q-projection.
Similarly, $[\mathbf{K}_{{\mathbf{X}^t}}, \mathbf{K}_{\mathbf{P}}]$ and $[\mathbf{V}_{{\mathbf{X}^t}}, \mathbf{V}_{\mathbf{P}}]$ denotes the output of the k-projection and v-projection layers.
$\mathbf{W}_{\{{q,k,v}\}} \in \mathbb{R}^{d \times d}$ and $\mathbf{b}_{\{{q,k,v}\}} \in \mathbb{R}^d$ denotes the weight and bias in the qkv-projection layer, respectively.
$[\mathbf{S}_{\mathbf{X}}, \mathbf{S}_{\mathbf{P}}] = softmax(\mathbf{Q}_{\mathbf{X}} [\mathbf{K}_{\mathbf{X}^t}, \mathbf{K}_{\mathbf{P}}]^{\top} / \sqrt{d})$ denotes the attention matrix after the MSA layer.
We derive the null space $\mathbf{U}_{1,0}$ and $\mathbf{U}_{2,0}$ of these two matrices through singular value
decomposition (SVD) following \cite{GPM, pgpICLR24, 2021nullspace}. 
After that, we get the projection matrices $\mathbf{U}_{1,0}\mathbf{U}_{1,0}^{\top}$ and $\mathbf{U}_{2,0}\mathbf{U}_{2,0}^{\top}$, which enables $\mathbf{P}$ to satisfy Eq.\ref{eq: null_space_definition}:

\begin{equation}\label{eq: optimize_null_space}
    \mathbf{P} \leftarrow
    \mathbf{P} - \lambda (\mathbf{U}_{2,0}\mathbf{U}_{2,0}^{\top})
    \mathbf{P}_{\mathcal{G}}(\mathbf{U}_{1,0}\mathbf{U}_{1,0}^{\top}), \forall \mathbf{P} \in \mathcal{P}_{sh} 
\end{equation}

\noindent where $\lambda$ denotes the learning rate and $\mathbf{P}_{\mathcal{G}}$ denotes the original gradient of prompt $\mathbf{P}$.

\subsection{Details of Evaluation Metrics}

Following \cite{ssaitCVPR24, l2pCVPR22, infloraCVPR24} and most continual learning methods based on pre-training, we evaluate our proposed method under two metrics:
the accuracy of all classes after learning the last session (Last-acc), 
and the averaged accuracy of all incremental sessions (Avg-acc).
Formally, the final Last-acc and Avg-acc are defined as:
\begin{equation*}
\begin{split}
&\text{Acc}_t = \frac{1}{t} \sum_{i=1}^{t}a_{t, i}, \quad
\text{Last-acc} = \text{Acc}_T,\\
&\text{Avg-acc} = \frac{1}{T} \sum_{t=1}^{T} \text{Acc}_t,
\end{split}
\end{equation*}
where \( T \) is the number of tasks, \( a_{T, i} \) is the accuracy of the \( T \)-th model on the \( i \)-th task samples, and \( a_{j, i} \) is the accuracy of the \( j \)-th model on the \( i \)-th task samples.

% Note that the aforementioned Last-acc is the commonly used metric in pre-training-based works.
% In addition to the final average accuracy, a few works also report mean average accuracy, which is defined as the mean value of the final average accuracies for all tasks.
The ``Last-acc'' metric is the primary metric that we should focus on, as it reflects the precision of classification in practice.

% For a fair comparison, we consistently report the final average accuracy for all the methods in our paper.

% Higher accuracy indicates better model performance, while lower forgetting signifies stronger stability (\textit{i.e.}, the ability to retain old knowledge).
% However, lower forgetting does not always lead to higher accuracy, as accuracy is also influenced by plasticity (\textit{i.e.}, the ability to learn new knowledge).
% Accuracy is the primary metric that we should focus on, as it reflects the precision of classification in practice.
